# Supplementary material for: X-IL: Exploring the Design Space of Imitation Learning Policies
Source: arXiv:2502.12330 source file (2025-02-19)
Supplement: Supplementary file 1 [file appendix_backbone_transformer.tex]

%%%%%%%%%%%%%%%%%%%%%%%%%%%%%%%%%%%%%%%%%%%%%%%%%%%%%%%%%%%%%%%%%%%%%%%%%%%%%%%%%%%%%%%%
\newcommand{\encoder}[1]{\textcolor{blue}{#1}}
\newcommand{\decoder}[1]{\textcolor{violet}{#1}}

\begin{table}[h]
\begin{center}
\begin{small}
\begin{sc}
\resizebox{0.8\linewidth}{!}{%
\begin{tabular}{l l|c|c|c|c|c|c}
\toprule
\textbf{Policy}
& \textbf{Transformer}
& \textbf{Layers}
& \textbf{Embeddings}
& \textbf{Heads}
& \textbf{Batch Size}
& \textbf{Learning rate}
& \textbf{Optimizer}
\\ 
\midrule
\multirow{2}{*}{DDPM}
& Dec
& 
& 
& 
& 
&
&
\\

& \encoder{Enc}-\decoder{Dec}
& 
& 
& 
& 
&
&
\\
\midrule
\multirow{2}{*}{BESO}
& Dec
& 
& 
& 
& 
&
&
\\

& \encoder{Enc}-\decoder{Dec}
& 
& 
& 
& 
&
&
\\
\midrule
\multirow{2}{*}{FM}
& Dec
& 
& 
& 
& 
&
&
\\
& \encoder{Enc}-\decoder{Dec}
& 
& 
& 
& 
&
&
\\
\bottomrule
\end{tabular}
}
\end{sc}
\end{small}
\end{center}
% \vskip -0.15in
    \caption{.. }
    % \vspace{-0.2cm}
\label{table:appendix_backbone_transformer}
\end{table}
%%%%%%%%%%%%%%%%%%%%%%%%%%%%%%%%%%%%%%%%%%%%%%%%%%%%%%%%%%%%%%%%%%%%%%%%%%%%%
